# Supplementary material for: Multi-Perspective Abstractive Answer Summarization
Source: arXiv:2104.08536 source file (2021-04-17)
Supplement: Supplementary file 1 [file appendix_separate.tex]

% %
% % File acl2021.tex
% %
% %% Based on the style files for EMNLP 2020, which were
% %% Based on the style files for ACL 2020, which were
% %% Based on the style files for ACL 2018, NAACL 2018/19, which were
% %% Based on the style files for ACL-2015, with some improvements
% %%  taken from the NAACL-2016 style
% %% Based on the style files for ACL-2014, which were, in turn,
% %% based on ACL-2013, ACL-2012, ACL-2011, ACL-2010, ACL-IJCNLP-2009,
% %% EACL-2009, IJCNLP-2008...
% %% Based on the style files for EACL 2006 by 
% %%e.agirre@ehu.es or Sergi.Balari@uab.es
% %% and that of ACL 08 by Joakim Nivre and Noah Smith

% \documentclass[11pt,a4paper]{article}
% \usepackage[hyperref]{acl2021}
% \usepackage{times}
% \usepackage{latexsym}
% \renewcommand{\UrlFont}{\ttfamily\small}


% \usepackage{graphicx}
% \usepackage{url}
% \usepackage{amsmath}
% \usepackage{breqn}
% \usepackage{makecell}
% \usepackage{tabularx}
% \usepackage{booktabs}
% \usepackage{multirow}
% \usepackage[colorinlistoftodos]{todonotes}
% \usepackage{textcomp}
% % \usepackage{comment}
% \usepackage{bm}
% \DeclareMathOperator*{\argmax}{argmax} %
% \newcommand{\specialcell}[2][c]{%
% \begin{tabular}[#1]{@{}c@{}}#2\end{tabular}}
% \usepackage{hyperref}
% \usepackage{amsmath}
% % This is not strictly necessary, and may be commented out,
% % but it will improve the layout of the manuscript,
% % and will typically save some space.
% \usepackage{microtype}
%   \definecolor{DarkGreen}{rgb}{0.2,0.5,0.2} 

% \newcommand\srini[1]{{\color{green}\textbf{ }{#1} }}
% \newcommand\xiaojian[1]{{\color{orange}\textbf{}{#1} }}
% \newcommand\mona[1]{{\color{blue}\textbf{ }{#1} }}
% \newcommand\alex[1]{{\color{red}\textbf{ }{#1} }}

% % This is not strictly necessary, and may be commented out,
% % but it will improve the layout of the manuscript,
% % and will typically save some space.
% \usepackage{microtype}

% \include{helpers}

% %\aclfinalcopy % Uncomment this line for the final submission
% %\def\aclpaperid{***} %  Enter the acl Paper ID here

% %\setlength\titlebox{5cm}
% % You can expand the titlebox if you need extra space
% % to show all the authors. Please do not make the titlebox
% % smaller than 5cm (the original size); we will check this
% % in the camera-ready version and ask you to change it back.

% \newcommand\BibTeX{B\textsc{ib}\TeX}

% \title{Instructions for ACL-IJCNLP 2021 Proceedings}

% \author{First Author \\
%   Affiliation / Address line 1 \\
%   Affiliation / Address line 2 \\
%   Affiliation / Address line 3 \\
%   \texttt{email@domain} \\\And
%   Second Author \\
%   Affiliation / Address line 1 \\
%   Affiliation / Address line 2 \\
%   Affiliation / Address line 3 \\
%   \texttt{email@domain} \\}

% \date{}
% % \title{AnswerSumm: Multi-perspective Answer Summarization \\ with Improved Coverage and Faithfulness }
% \title{Multiperspective Abstractive Answer Summarization}
% \begin{document}
% % \maketitle

% \appendix
% \input{91-appendix}





% % \bibliographystyle{acl_natbib}
% % \bibliography{acl2021}




% \end{document}
